# Supplementary material for: Amorphous Entangled Active Matter
Source: arXiv:2207.03665 source file (2022-07-08)
Supplement: Supplementary file 1 [file sm1.tex]

\documentclass[aps,reprint,pre,twocolumn,groupedaddress,showkeys,10pt,amsmath,amssymb]{revtex4-1}
\usepackage[dvipsnames]{xcolor} %allow colored comments

%\documentclass[aps,prl,preprint,superscriptaddress]{revtex4-1}
%\documentclass[aps,prl,reprint,groupedaddress]{revtex4-1}
%diameter char/include figure files/align table columns on decimal point/bold math
\usepackage{wasysym,graphicx,dcolumn,bm}

\usepackage{romannum}
\usepackage{filecontents}
% You should use BibTeX and apsrev.bst for references
% Choosing a journal automatically selects the correct APS
% BibTeX style file (bst file), so only uncomment the line
% below if necessary.
