# Supplementary material for: Amorphous Entangled Active Matter
Source: arXiv:2207.03665 source file (2022-07-08)
Supplement: Supplementary file 3 [file sm3.tex]

\begin{acknowledgments}
We thank Akash Vardhan for experimental assistance, Dana Randall, Andr\'{e}a W.~Richa, and Paul Umbanhowar for helpful discussions.
\end{acknowledgments}
