# Supplementary material for: Amorphous Entangled Active Matter
Source: arXiv:2207.03665 source file (2022-07-08)
Supplement: Supplementary file 4 [file sm4.tex]

\bibliographystyle{apsrev4-1} %the RSC's .bst file
