# Supplementary material for: Amorphous Entangled Active Matter
Source: arXiv:2207.03665 source file (2022-07-08)
Supplement: Supplementary file 5 [file SI.tex]

%%!TEX root = main.tex

%remove one '%' from above line and comment below to use in full document
%remove magic references and uncomment true references when making full document
%%%%UNCOMMENT IF NOT RUN UNDER MAIN TEXT%%%%%%%%%%%%%%%%%%%%%%%%%%%%%%%%%
%\RequirePackage[usenames,dvipsnames,array,table]{xcolor} %allow colored comments

% \documentclass[aps,reprint,prl,onecolumn,groupedaddress,showkeys,10pt,amsmath,amssymb]{revtex4-1}
% \usepackage[dvipsnames]{xcolor} %allow colored comments

% %\documentclass[aps,prl,preprint,superscriptaddress]{revtex4-1}
% %\documentclass[aps,prl,reprint,groupedaddress]{revtex4-1}
% %diameter char/include figure files/align table columns on decimal point/bold math
% \usepackage{wasysym,graphicx,dcolumn,bm}

% \newcommand{\redcomment}[1]{\textcolor{OrangeRed}{#1}}
% \newcommand{\bluecomment}[1]{\textcolor{Cerulean}{#1}}
% \newcommand{\greencomment}[1]{\textcolor{ForestGreen}{#1}}

% \newcommand{\beginsupplement}{%
%         \setcounter{table}{0}
%         \renewcommand{\thetable}{S\arabic{table}}%
%         \setcounter{figure}{0}
%         \renewcommand{\thefigure}{S\arabic{figure}}%
%      }
     
% \usepackage{romannum}

% You should use BibTeX and apsrev.bst for references
% Choosing a journal automatically selects the correct APS
% BibTeX style file (bst file), so only uncomment the line
% below if necessary.
%\bibliographystyle{apsrev4-1}
%SI section
% \begin{document}
%%%%UNCOMMENT IF NOT RUN UNDER MAIN TEXT%%%%%%%%%%%%%%%%%%%%%%%%%%%%%%%%%
%%%%%%%%%%%%%%
\section{\label{sec:SI} Supporting Information (SI)}
the exact dimensions of the three-tiered container are listed below.

%Each tier is composed of two levels of planks rotated to make a closed cylinder. The bottom levels are tilted inwardly and the top levels tilted out at and angle of $30^\circ$. The maximum radius of each tier is \redcomment{add radius of each tier here} $[r1,r2,r3]$m from the bottom to top tiers respectively.

\redcomment{find new word instead of activity}

%\redcomment{find new order parameter to correlate mechanical aspects}

\redcomment{With a robotic collective, it is possible to create a material which could generate multiple desired responses, lessening dependence on single use design paradigms}
