# Supplementary material for: Amorphous Entangled Active Matter
Source: arXiv:2207.03665 source file (2022-07-08)
Supplement: Supplementary file 7 [file sm3.tex]

\section*{Conflicts of interest}
In accordance with our policy on \href{http://www.rsc.org/journals-books-databases/journal-authors-reviewers/author-responsibilities/#code-of-conduct}{Conflicts of interest} please ensure that a conflicts of interest statement is included in your manuscript here.  Please note that this statement is required for all submitted manuscripts.  If no conflicts exist, please state that ``There are no conflicts to declare''.

\section*{Acknowledgements}
We thank Akash Vardhan for experimental assistance, Dana Randall, Andr\'{e}a W.~Richa, and Paul Umbanhowar for helpful discussions.

%%%END OF MAIN TEXT%%%

%The \balance command can be used to balance the columns on the final page if desired. It should be placed anywhere within the first column of the last page.

\balance

%If notes are included in your references you can change the title from 'References' to 'Notes and references' using the following command:
%\renewcommand\refname{Notes and references}

%%%REFERENCES%%%
